# Supplementary material for: Discourse Understanding and Factual Consistency in Abstractive Summarization
Source: arXiv:1907.01272 source file (2021-04-09)
Supplement: Supplementary file 1 [file old_appendix.tex]

\begin{table}
\begin{center}
\resizebox{\columnwidth}{!}{%
    \begin{tabular}{rrrr}
    \toprule
    Discriminator Evaluation & Eval Task & \% Transformer-G & \% Transformer-D \\ \toprule
     & 32.5  & 33.5 & 49.5\\ \toprule
     Turing Evaluation & \% Gold Ranked First & \% Gold Ranked Last & \% \model~Selection > Gold\\  \toprule
         & Select First  & 23.5 & 29.0  \\
    % Abstractiveness  & 50.9 & 28.3 & 20.8\\ 
    & Select Last & 31.0 & 33.5 \\
    %Select Overall & 13.5  & 13.0  \\
    \bottomrule
    \end{tabular}
}
\caption{MTurk Discriminator and Turing evaluation results. Comparison between Transformer generated abstracts and gold abstracts.}
\label{table:turing}
\end{center}
\end{table}
